# Supplementary material for: On the representation of capsizing in iceberg models
Source: arXiv:1702.06870 source file (2017-02-22)
Supplement: Supplementary file 1 [file Rolling_SI.pdf]

# Supplementary Information

## On the representation of capsizing in iceberg models

By Till J.W. Wagner, Alon A. Stern, Rebecca W. Dell, and Ian Eisenman

## Derivation of Rolling Stability Criterion

Consider a cuboid iceberg of height, $H$, and width, $W$, with aspect ratio $\epsilon \equiv W/H$. The iceberg is taken to float at isostatic equilibrium, with densities of water $\rho_w$ and ice $\rho_i$, and density ratio $\alpha \equiv \rho_i/\rho_w$. For a given angle of rotation, $\theta$, the horizontal position of the center of gravity, $x_g$, is found to be as follows (here, the $x$-axis origin is chosen to be located at the left hand intersection of the iceberg and sea level, see Fig S1):

$$x_g/H = \frac{\epsilon}{2\cos\theta} - \left(\alpha - \frac{1}{2}\right)\sin\theta. \tag{S1}$$

The center of buoyancy, $x_b$, is readily derived by sectioning the submerged area of the iceberg into a triangle and a square, as indicated in Fig S1. We have

$$x_b = \frac{x_1 A_1 + x_2 A_2}{A_1 + A_2}. \tag{S2}$$

We find

$$x_1/H = \frac{\epsilon}{3}\left(\cos\theta + \frac{1}{\cos\theta}\right), \qquad x_2/H = \frac{\epsilon}{2\cos\theta}\left(1 - \frac{1}{2}\sin^2\theta\right) - \frac{\alpha}{2}\sin\theta \tag{S3}$$

and

$$A_1/H^2 = \frac{\epsilon^2}{2\tan\theta}, \qquad A_2/H^2 = \epsilon\left(\alpha - \frac{1}{2}\epsilon\tan\theta\right). \tag{S4}$$

Note that $A_1 + A_2 = H^2\epsilon\alpha$. Substituting (S3) and (S4) into (S2) gives

$$x_b/H = \frac{1}{24\alpha}\left[\left(\epsilon^2 - 12\alpha^2\right)\sin\theta + \epsilon\sec\theta\left(12\alpha + \epsilon\tan\theta\right)\right]. \tag{S5}$$

Finally, the horizontal distance between the centers of gravity and buoyancy is then given as

$$\Delta x \equiv x_b - x_g = \frac{H}{24\alpha}\left\{\left[12\alpha\left(\alpha - 1\right) + \epsilon^2\right]\sin\theta + \epsilon^2\sec\theta\tan\theta\right\}, \tag{S6}$$

which corresponds to equation (1) of the main text.

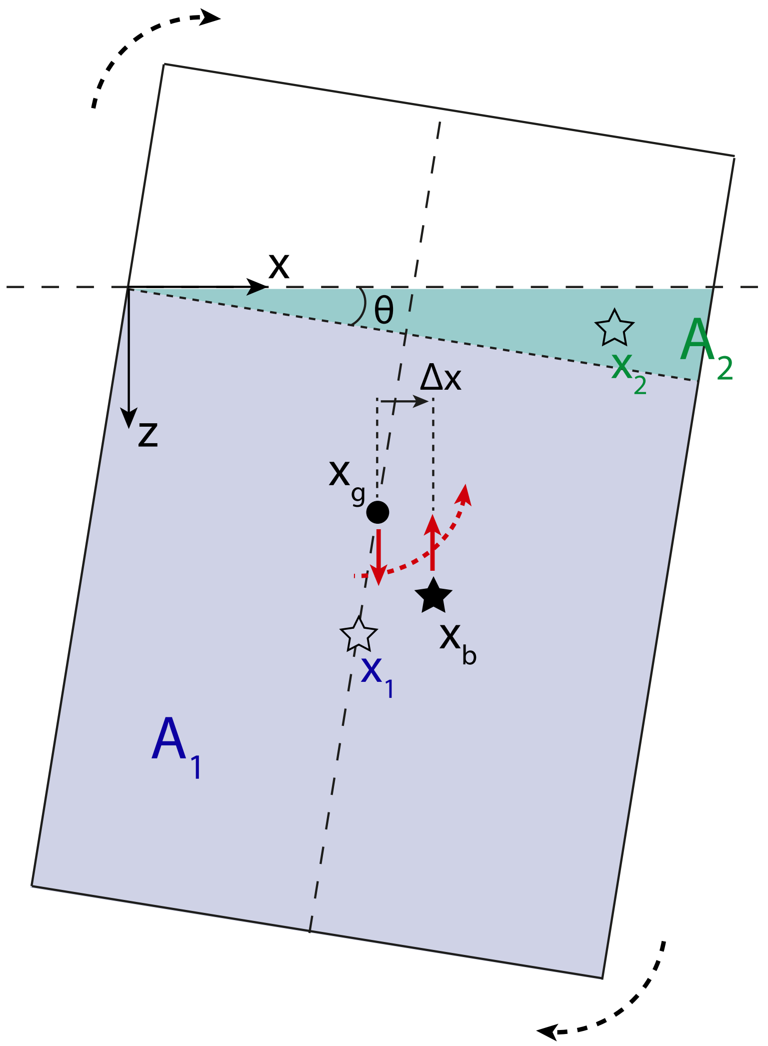


Figure S1. Schematic of an iceberg rotated by an angle $\theta$. Indicated in blue and green are the two submerged areas, with auxiliary centers of buoyancy (☆) used to compute the overall center of buoyancy (★). Also shown is the center of gravity (•), and the horizontal offset between the centers of buoyancy and gravity, $\Delta x = x_b - x_g$. The red arrows indicate the forces of gravity and buoyancy (solid) and the resulting torque (dashed). Since $\Delta x > 0$ in this case, the resulting torque counteracts the rotation $\theta$, leading to a stable, self-righting, iceberg configuration.
